# Supplementary material for: StoryMI: Steerable Multi-Agent Therapeutic Dialogue Generation
Source: arXiv:2605.27393 source file (2026-04-18)
Supplement: Supplementary file 1 [file appendix.tex]

% this file is called up by thesis.tex
% content in this file will be fed into the main document

%: ----------------------- name of chapter  -------------------------
\section{Appendix} % top level followed by section, subsection

% \begin{figure*}[t]
%     \centering
%     \includegraphics[width=0.95\linewidth]{ACL template/latex/figs/ACL26_MIMAS_F2_therapist.png}
%     \caption{Therapist Utterance Generation}
%     \label{fig:therapistgen}
% \end{figure*}

% ---------------------------------------------------------------------------
%: ----------------------- end of thesis sub-document ------------------------
% ---------------------------------------------------------------------------
